# Supplementary material for: Towards Evaluating and Building Versatile Large Language Models for Medicine
Source: arXiv:2408.12547 source file (2024-09-05)
Supplement: Supplementary file 1 [file supplementary.tex]

% \documentclass[10pt, letter, onecolumn]{arxiv}


% \usepackage{kantlipsum, lipsum}
% \usepackage{dm-colors}
% \usepackage{amsmath}
% \usepackage{pstricks, pst-node}
% \usepackage{verbatim}
% \usepackage{multirow}
% \usepackage{scalerel}
% \usepackage{booktabs}
% \usepackage{enumitem}
% \usepackage{xspace}
% \usepackage{bm}
% \usepackage{bbm}
% \usepackage{mathtools}
% \usepackage{soul}
% \usepackage{epsfig}
% \usepackage{graphicx}
% \usepackage{amssymb}
% \usepackage{colortbl}
% \usepackage{csquotes}
% \usepackage{setspace}
% \usepackage{colortbl}
% \usepackage{bbding}
% \usepackage{threeparttable}
% \usepackage{tabularx,ragged2e}
% \usepackage{placeins}
% \usepackage{bbding}
% %\definecolor{darkpastelgreen}{rgb}{0.01, 0.75, 0.24}
% \definecolor{darkpastelgreen}{rgb}{0.13, 0.55, 0.13}
% %\definecolor{darkpastelred}{rgb}{0.76, 0.23, 0.13}
% \definecolor{darkpastelred}{rgb}{0.55, 0.13, 0.13}
% \definecolor{mygray}{rgb}{0.85, 0.85, 0.85}
% % \usepackage{lstlisting}
% %\usepackage[symbol]{footmisc}
% \usepackage[hang,flushmargin]{footmisc}

% % \usepackage[bibstyle=nature,citestyle=numeric-comp,%
% %             natbib=true,backend=biber,maxbibnames=99,%
% %             giveninits=false,sorting=none]{biblatex}
% % \usepackage{natbib}
% \usepackage{nameref}
% \usepackage{varioref}
% \usepackage{amssymb}% http://ctan.org/pkg/amssymb
% \usepackage{pifont}% http://ctan.org/pkg/pifont
% \newcommand{\cmark}{\ding{51}}%
% \newcommand{\xmark}{\ding{55}}%

% \usepackage[pagebackref=false,breaklinks=false,%
%             colorlinks=true,bookmarks=true,citecolor=ourdarkblue,%
%             urlcolor=ourdarkblue,linkcolor=ourdarkblue]{hyperref}
% \usepackage[noabbrev,capitalize]{cleveref}
% \usepackage{etoc}
% %\usepackage{lineno}
% \usepackage{algorithm}
% \usepackage{algpseudocode}
% %\addbibresource{references.bib}
% %\renewcommand*{\bibfont}{\linespread{0.8}\footnotesize}
% % \usepackage[table]{xcolor} % 确保加载了xcolor包
% % \definecolor{mygray}{gray}{0.9} % 在这里定义颜色mygray

% \graphicspath{{figures/}}

% \newcommand{\weidi}[1]{{\textcolor{magenta}{[weidi: #1]}}}
% \newcommand{\xiaoman}[1]{{\textcolor{cyan}{[xiaoman: #1]}}}
% \newcommand{\chaoyi}[1]{{\textcolor{blue}{[chaoyi: #1]}}}
% \newcommand{\qiaoyu}[1]{{\textcolor{brown}{[qiaoyu: #1]}}}
% \newcommand{\weike}[1]{{\textcolor{orange}{[keke: #1]}}}
% \newcommand{\pengcheng}[1]{{\textcolor{red}{[Pengcheng: #1]} }}


% \newcommand{\todo}[1]{\textcolor{blue}{\textbf{TODO:} (#1)}}
% \newcommand{\mn}[1]{\textcolor{blue}{{(MN: #1)}}}
% \newcommand{\one}[1]{\mathbbm{1}_{[#1]}}
% \newcommand{\figref}[1]{Fig.~\ref{#1}}
% \newcommand{\tabref}[1]{Tab.~\ref{#1}}
% \newcommand{\secref}[1]{Sec.~\ref{#1}}
% \newcommand{\AlgRef}[1]{Algorithm~\ref{#1}}
% \newcommand{\equref}[1]{Equ.~(\ref{#1})}

% \newenvironment{rednote}{\par\color{red}}{\par}


% \def\eg{{\em e.g.,}}
% \def\ie{{\em i.e.,}}
% \def\vs{{\em vs.~}}
% \def\etc{{\em etc}\xspace}
% \def\etal{{\em et al.}\xspace}


% \title{\Large{\Large{Towards Building Multilingual Language Model for Medicine}~(Supplementary Material)}}


% % -------------  Authors ----------------------
% % \author[$\ast$,1]{Anonymous Author List \weidi{give name list}}

% % % -------------  Authors ----------------------
% \author[$\ast$,1,2]{Pengcheng Qiu} %#1
% \author[$\ast$,1,2]{Chaoyi Wu} %#1
% \author[1,2]{Xiaoman Zhang} %#
% \author[1,2]{Weixiong Lin} %#1
% \author[1]{Haicheng Wang} %#1
% \author[1,2]{\\ \vspace{0.1cm} Ya Zhang}
% \author[1,2,$\dag$]{Yanfeng Wang} 
% \author[1,2,$\dag$]{Weidi Xie}
% \affil[1]{\normalsize Shanghai Jiao Tong University \hspace{1cm}}

% \affil[2]{\normalsize Shanghai AI Laboratory \authorcr

% \url{https://github.com/MAGIC-AI4Med/MMedLM}

% }

% \renewcommand{\correspondingauthor}[1]{$\ast$~Equal contributions. \\ $\dag$~Corresponding author. Email addresses: qiupengcheng@pjlab.org.cn, \{wtzxxxwcy02, weidi\}@sjtu.edu.cn}


% \begin{document}
% %\begin{refsection}
% % \linenumbers 
% \begin{abstract}
% \end{abstract}
% \maketitle

% % ------------ SECTIONS ---------------------

% % ========== Edit your name here

% %\setlength\bibitemsep{3pt}
% %\printbibliography
% %\balance

% \appendix

% \input{content_npj/06_Appendix}

% % \clearpage
% % \bibliographystyle{sn-mathphys} % We choose the "plain" reference style
% % \bibliography{references} % Entries are in the refs.bib file


% %\end{refsection}
% \end{document}
